# Supplementary material for: Extended Radial Basis Function Controller for Reinforcement Learning
Source: arXiv:2009.05866 source file (2020-12-09)
Supplement: Supplementary file 1 [file 0_supplementary.tex]

{\large \textbf{Supplement Note on Experimental Validation with Real Data}}

Due to the physical set-ups being inaccessible, we have not validated our extended RBF controller design with real data. 

We are, however, confident that our method will work on real physical environments, because of the following.

\begin{itemize}
    \item The theoretical design has been tested extensively in three different OpenAI gym simulation environments, and have performed in line with theory.
    \item We do not expect any transfer learning problem such as Sim-to-Real, as neither our controller design nor our learning is domain dependent. 
    \item We expect some modelling errors in the physical set-up, such as measurement errors and friction (simulation systems have been frictionless). However, as shown in Section 4, our extended RBF controller is robust against such errors by design. Furthermore, we could reparameterise the linear controllers accordingly should the frictional force be sizeable.
\end{itemize}

In the event that the physical experimental set-ups become accessible again, we would do the following.

\begin{itemize}
    \item Perform experiments similar to those of the simulation in the real-world Swing-up Pendulum and Cartpole environments.
    \item We would not conduct any physical experiments for the Mountain Car environment since this is unavailable.
\end{itemize}
